# Supplementary material for: Chaos Gaussian Splatting: Polynomial Regression with Gaussian Splats for Chaotic Maps with Gradient Discontinuities
Source: arXiv:2611.35989 source file (2026-11-26)
Supplement: Supplementary file 1 [file supp_labels_arxiv.tex]

% generated by make_journal.py from gscn_supplement.aux (tables the arXiv version omits) -- do not edit
\makeatletter
\@namedef{supp@sec:networks-full}{S1}
\@namedef{supp@eq:coherence}{1}
\@namedef{supp@eq:stretch}{3}
\@namedef{supp@sec:safeguards}{S2}
\@namedef{supp@eq:guard}{5}
\@namedef{supp@sec:closedloop}{S3}
\@namedef{supp@eq:valhorizon}{6}
\@namedef{supp@sec:polyrelation}{S4}
\@namedef{supp@tab:polymodels}{S1}
\@namedef{supp@sec:stencil-method}{S5}
\@namedef{supp@sec:cost-full}{S6}
\@namedef{supp@sec:v4-longcost}{S7}
\@namedef{supp@eq:views}{7}
\@namedef{supp@sec:baselines-full}{S8}
\@namedef{supp@tab:regimes}{S2}
\@namedef{supp@tab:cost}{S3}
\@namedef{supp@fig:budget}{S1}
\@namedef{supp@fig:budget-cost}{S2}
\@namedef{supp@tab:budget-cost}{S4}
\@namedef{supp@tab:budget-targets}{S5}
\@namedef{supp@tab:budget-small}{S6}
\@namedef{supp@sec:henon}{S17}
\@namedef{supp@sec:flows}{S18}
\@namedef{supp@tab:flows}{S7}
\@namedef{supp@fig:santafe}{S3}
\@namedef{supp@tab:santafe}{S8}
\@namedef{supp@sec:dysts}{S23}
\@namedef{supp@fig:dysts}{S4}
\@namedef{supp@sec:longr2}{S24}
\@namedef{supp@tab:longr2}{S9}
\@namedef{supp@fig:long-smooth}{S5}
\@namedef{supp@fig:long-kinked}{S6}
\@namedef{supp@fig:noise}{S7}
\@namedef{supp@tab:noise-full}{S10}
\@namedef{supp@tab:abl-dims}{S11}
\@namedef{supp@sec:noise-full}{S30}
\@namedef{supp@sec:l63}{S32}
\@namedef{supp@tab:l63}{S12}
\@namedef{supp@sec:l96}{S33}
\@namedef{supp@sec:smooth-full}{S34}
\@namedef{supp@tab:fresh910}{S13}
\@namedef{supp@tab:fresh11}{S14}
\@namedef{supp@tab:v4-robust}{S15}
\@namedef{supp@tab:fresh-rollouts}{S16}
\@namedef{supp@tab:ladder910}{S17}
\@namedef{supp@tab:pointdist910}{S18}
\@namedef{supp@sec:fresh-full}{S42}
\@namedef{supp@sec:fairness-more}{S43}
\@namedef{supp@tab:cheat}{S19}
\@namedef{supp@tab:criticisms}{S20}
\@namedef{supp@sec:fairness-full}{S46}
\@namedef{supp@sec:hidden}{S48}
\@namedef{supp@sec:extra-baselines}{S52}
\@namedef{supp@tab:extra-baselines}{S21}
\@namedef{supp@sec:polyprop-fresh}{S53}
\@namedef{supp@tab:polyprop}{S22}
\@namedef{supp@fig:kink-errors}{S8}
\@namedef{supp@sec:machine}{S55}
\@namedef{supp@tab:datasets}{S23}
\@namedef{supp@tab:baselines}{S24}
\@namedef{supp@tab:complexity}{S25}
\@namedef{supp@tab:heldout2}{S26}
\@namedef{supp@tab:abl-components}{S27}
\@namedef{supp@tab:learning}{S28}
\@namedef{supp@app:tables}{S57}
\@namedef{supp@tab:maps-baselines}{S29}
\@namedef{supp@tab:l96}{S30}
\@namedef{supp@app:v4spec}{S58}
\makeatother
